# Supplementary material for: Continual Learning of Context-dependent Processing in Neural Networks
Source: arXiv:1810.01256 ancillary file (2021-06-27)
Supplement: Supplementary file 1 [file SUPPLEMENTARY_MATERIALS.pdf]

---

# Supplementary Material For Continuous Learning of Context-dependent Processing in Neural Networks

Guanxiong Zeng<sup>1,2,\*</sup>, Yang Chen<sup>1,\*</sup>, Bo Cui<sup>1,2</sup> and Shan Yu<sup>1,2,3,†</sup>

<sup>1</sup>Brainnetome Center and National Laboratory of Pattern Recognition, Institute of Automation, Chinese Academy of Sciences, 100190 Beijing, China.

<sup>2</sup>University of Chinese Academy of Sciences, 100049 Beijing, China.

<sup>3</sup>CAS Center for Excellence in Brain Science and Intelligence Technology, Chinese Academy of Sciences, 100190 Beijing, China.

\* These authors contributed equally to this work.

† Correspondence; [shan.yu@nlpr.ia.ac.cn](mailto:shan.yu@nlpr.ia.ac.cn)

## SUPPLEMENTARY TEXT

### I. Comparison of OWM and CAB

OWM and CAB were separately proposed to the same purpose, that is, to avoid catastrophic forgetting by training the network along the direction orthogonal to the inputs of learned tasks. However, as demonstrated below, there are key differences in the two approaches, leading to substantial performance gap between them.

In order to shield previously learned knowledge by training the network in a direction orthogonal to the space spanned by previous inputs, the most important step is to construct a proper orthogonal projector. The design of the projector differentiates OWM from CAB significantly. OWM construct the orthogonal projector as  $\mathbf{A}(\mathbf{A}^T \mathbf{A})^{-1} \mathbf{A}^T$ , where  $\mathbf{A}$  contains previous inputs as its columns. The construction of this orthogonal projector is mathematically sound [1–3]. On top of this exact solution of orthogonal projector, we introduced the term of  $\alpha \mathbf{I}$  to change the projector as  $\mathbf{A}(\mathbf{A}^T \mathbf{A} + \alpha \mathbf{I})^{-1} \mathbf{A}^T$ . This enables us to choose to protect the entire subspace spanned by previous inputs or part of it to avoid the influence of noise [3, 4].

In CAB, the construction of the projector was based on the Conceptor, which was defined as the  $\mathbf{C}$  that minimizes the loss function of  $\mathbb{E}_x[||\mathbf{x} - \mathbf{C}\mathbf{x}||^2] + \alpha^{-2} ||\mathbf{C}||_{fro}$  (Eq. 1 in [5]). The first item, i.e.,  $\mathbb{E}_x[||\mathbf{x} - \mathbf{C}\mathbf{x}||^2]$  in this loss function is actually all what we need to construct a proper projector. Obviously, the linear system  $\mathbf{x} = \mathbf{C}\mathbf{x}$  is compatible and may has infinite solutions especially when  $\mathbf{x}$  doesn't span all its possible space, which is always the case for the tasks learned earlier in sequential learning. Actually, the equation  $\mathbf{x} = \mathbf{C}\mathbf{x}$  has a unique and exact solution under the constraint of minimum norm of  $\mathbf{C}$ , i.e.,  $\min_{\mathbf{x}-\mathbf{C}\mathbf{x}=0} ||\mathbf{C}||$ . The equation  $\mathbf{x} = \mathbf{C}\mathbf{x}$  is equivalent to

$$\mathbf{C}\mathbf{A} = \mathbf{A} \tag{S1}$$

where  $\mathbf{A}$  is the matrix consisted of data vectors as its columns as defined in our manuscript. To solve the Eq.S1, one can vectorize Eq.S1 and reorganize it as the following [1, 6]

$$(\mathbf{I} \otimes \mathbf{A}^T) \text{vec}(\mathbf{C}) = \text{vec}(\mathbf{A}) \tag{S2}$$

where  $\otimes$  denotes the Kronecker product and  $\text{vec}(\mathbf{C}) = \text{vec}([\mathbf{c}_1, \mathbf{c}_2, \dots, \mathbf{c}_n]) = [\mathbf{c}_1^T, \mathbf{c}_2^T, \dots, \mathbf{c}_n^T]^T$  (so to  $\text{vec}(\mathbf{A})$ ). To find the minimum norm solution [1] of Eq.S2. It will lead to  $\mathbf{C} = \mathbf{A}(\mathbf{A}^T \mathbf{A})^{-1} \mathbf{A}^T$ , which is the orthogonal projector used in OWM. However, CAB does not solve the equation of  $\mathbf{A}\mathbf{x} = \mathbf{x}$  exactly. Instead, it constructs the projector based on minimizing the loss function cited above. The second term, i.e.,  $\alpha^{-2} \|\mathbf{A}\|_{fro}$ , in the loss function inevitably introduces error to the projector. In other words, the solution (Eq.S2 in their paper) that minimizes their loss function can't provide accurate protection of previous input space. It would lead to errors in updating the weights, eventually resulting in unwanted interference with previously learned tasks and compromising the ability of continuous learning. Furthermore, it is noteworthy that in the limiting case of  $\alpha^{-2}$  approaching zero, the Conceptor would be ill-defined due to the fact that for earlier tasks in continual learning the matrix  $\mathbf{R}$  would not be of full rank and, therefore, non-invertible. So, the projector in CAB will not approach the one used in OWM by changing the parameters.

Further, we demonstrate with MNIST inputs that the above-mentioned theoretical difference indeed leads to substantial error in the orthogonal projector of CAB, in comparison to OWM. To demonstrate that the difference in projector construction explained above will lead to difference in accuracy that matters for real data. We compared the error between the original inputs and that after the operation of the projector,  $\frac{1}{N} \sum_{i=1}^N \sqrt{\frac{1}{s} \|\mathbf{x}_i - \mathbf{x}_i^{pro}\|^2}$ ,  $\mathbf{x}^{pro} = (\mathbf{I} - \mathbf{P}^{owm})\mathbf{x}$  or  $\mathbf{C}\mathbf{x}$ .  $N$  is the number of data samples and  $s$  is the size/dimension of each input. More accurate projector will lead to smaller difference between the two, and vice versa. In Fig. S3, we plotted the errors for CAB and OWM with different choices of parameters. by taking image data of number "0" and "1" in MNIST dataset as an example. The projection by OWM was more precise (by a few orders of magnitudes) over a wide range of possible values of parameter.

To further investigate the influence of above difference of OWM in overcoming catastrophic interference compared to CAB, we tested these two methods in 10-disjoint MNIST task. That is, the network needs to learn recognizing digits from 0 to 9, one class at a time. In Fig. S4, we can see that the with more digits learned, the performance gap between these two methods enlarged, which was larger than 10% after learning all 10 digits. This is consisted with our above analyses that OWM can provide a much better protection to previously learned knowledge in the network.

To further examine the properties of the method, we analyzed the learning curve of OWM to demonstrate how much forgetting occurred for the earlier tasks. In Fig. S5, we show the learning curve of OWM, CAB and SGD on the 2-disjoint MNIST task (Task A, classifying 0,1,2,3,4; Task B, classifying 5,6,7,8,9). It can be seen from the learning curves that after the training of the Task B, OWM showed minimum decrease in the performance of the Task A, indicating a slight "forgetting" of the earlier task. In contrast, CAB showed more pronounced forgetting, consistent with our analysis that CAB is inferior in protecting learned knowledge. Finally, without any mechanism to prevent catastrophic forgetting (SGD), Task A was completely forgotten after the completion of learning the Task B.

## II. Relation of OWM and online EWC.

The loss function of online EWC can be organized as:

$$L = L_{err} + \frac{1}{2} \lambda L_{reg} \quad (\text{S3})$$

where

$$L_{reg} = \sum_i (\theta_i - \theta_i^*)^T \mathbf{F}_i (\theta_i - \theta_i^*) \quad (\text{S4})$$

$\theta_i$  and  $\theta_i^*$  are the input weights of neuron  $i$  in current task and last task, respectively, and  $\mathbf{F}_i$  is the corresponding Fisher information matrix. Take gradients on both sides of Eq.S3 for  $\theta_i$

$$\begin{aligned}\nabla_{\theta_i} L &= \nabla_{\theta_i} L_{err} + \frac{1}{2} \lambda \nabla_{\theta_i} L_{reg} \\ &= \nabla_{\theta_i} L_{err} + \lambda \mathbf{F}_i (\theta_i - \theta_i^*) \\ &\approx \nabla_{\theta_i} L_{err} - \lambda \mathbf{F}_i \nabla_{\theta_i} L_{err} \\ &= (\mathbf{I} - \lambda \mathbf{F}_i) \nabla_{\theta_i} L_{err}\end{aligned}\tag{S5}$$

Before the activation function, the input-output map of the  $i^{th}$  neuron can be viewed as a linear model with white noises (errors)

$$y_i = \theta_i^T \mathbf{x}_i + \epsilon_i \tag{S6}$$

There is a relationship between  $\mathbf{F}_i$ , the Fisher's information matrix of  $\theta_i$  and  $\mathbf{R}_i$ , the correlation matrix of its input  $\mathbf{x}_i$ ,

$$\mathbf{F}_i = \frac{1}{\sigma^2} \mathbf{R}_i \tag{S7}$$

where  $\sigma$  is the variance of white noise (or error)  $\epsilon_i$ . If we define the orthogonal projection matrix as  $\mathbf{P}_i^{(owm)} = \mathbf{I} - (1 + \alpha) \mathbf{A} (\mathbf{A}^T \mathbf{A} + \alpha \mathbf{I})^{-1} \mathbf{A}^T$ , and provided that  $\lambda \sim \sigma^2$ , then to substitute Eq.S7 into Eq.S5 we can derive the following

$$\begin{aligned}\nabla_{\theta_i} L &= (\mathbf{I} - \lambda \mathbf{F}_i) \nabla_{\theta_i} L_{err} \\ &= (\mathbf{I} - \frac{\lambda}{\sigma^2} \mathbf{R}_i) \nabla_{\theta_i} L_{err} \\ &\approx \lim_{\alpha \rightarrow \infty} \mathbf{P}_i^{(owm)} \Delta \theta_i^{bp}\end{aligned}\tag{S8}$$

indicating that EWC can be approximated as a special case of OWM in the limit of  $\alpha$  approaching the infinity.

## REFERENCES FOR SUPPLEMENTARY MATERIAL

- [1] Adi Ben-Israel and Thomas NE Greville. *Generalized inverses: theory and applications*, volume 15. Springer Science & Business Media, 2003.
- [2] Simo Puntanen. Projection matrices, generalized inverse matrices, and singular value decomposition by haruo yanai, kei takeuchi, yoshio takane. *International Statistical Review*, 79(3):503–504, 2011.
- [3] Simon S Haykin. *Adaptive filter theory*. Pearson Education India, 2008.
- [4] G. V. Moustakides. Study of the transient phase of the forgetting factor rls. *Ieee Transactions on Signal Processing*, 45(10):2468–2476, 1997.
- [5] Xu He and Herbert Jaeger. Overcoming catastrophic interference using conceptor-aided backpropagation. In *International Conference on Learning Representations*, 2018.
- [6] Marvin Marcus and Henryk Minc. *A survey of matrix theory and matrix inequalities*, volume 14. Courier Corporation, 1992.
- [7] Ian J Goodfellow, Mehdi Mirza, Da Xiao, Aaron Courville, and Yoshua preprint arXiv: Bengio. An empirical investigation of catastrophic forgetting in gradient-based neural networks. 2013.
- [8] James Kirkpatrick, Razvan Pascanu, Neil Rabinowitz, Joel Veness, Guillaume Desjardins, Andrei A. Rusu, Kieran Milan, John Quan, Tiago Ramalho, Agnieszka Grabska-Barwinska, Demis Hassabis, Claudia Clopath, Dharshan Kumaran, and Raia Hadsell. Overcoming catastrophic forgetting in neural networks. *Proceedings of the National Academy of Sciences of the United States of America*, 114(13):3521–3526, 2017.
- [9] Sang-Woo Lee, Jin-Hwa Kim, Jaehyun Jun, Jung-Woo Ha, and Byoung-Tak Zhang. Overcoming catastrophic forgetting by incremental moment matching. In *Advances in Neural Information Processing Systems*, pages 4652–4662, 2017.
- [10] Friedemann Zenke, Ben Poole, and Surya Continual learning through synaptic intelligence. 2017.
- [11] K. M. He, X. Y. Zhang, S. Q. Ren, J. Sun, and Ieee. *Deep Residual Learning for Image Recognition*, pages 770–778. IEEE Conference on Computer Vision and Pattern Recognition. Ieee, New York, 2016.
- [12] Tijmen Tieleman and Geoffrey Hinton. Lecture 6.5-rmsprop: Divide the gradient by a running average of its recent magnitude. *COURSERA: Neural networks for machine learning*, 4(2):26–31, 2012.

## SUPPLEMENTARY FIGURES AND TABLES

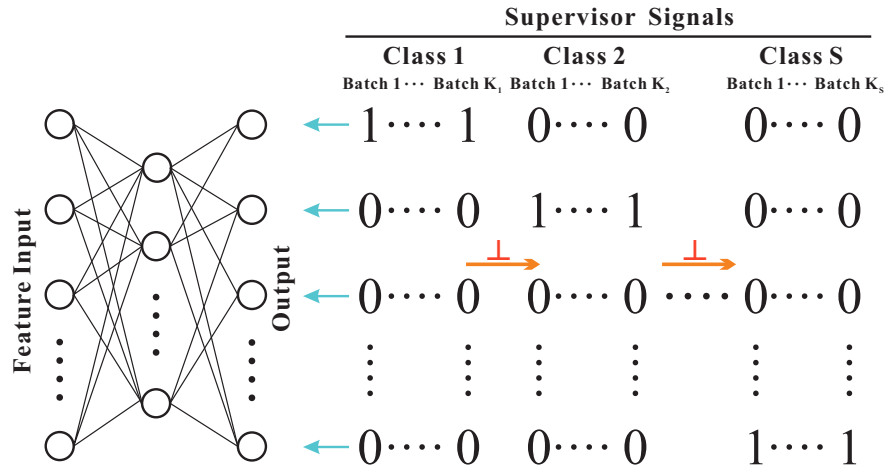

**Figure S1. Schematic diagram showing the procedure for sequential learning using OWM.** There were classes of data to be learned. Training samples of each class were sequentially fed to the neural network. The samples of the  $i^{th}$  class were further divided into  $K_i$  batches for training. The symbol “ $\perp$ ” denotes the application of the orthogonal projector  $P$  (see Methods for details).

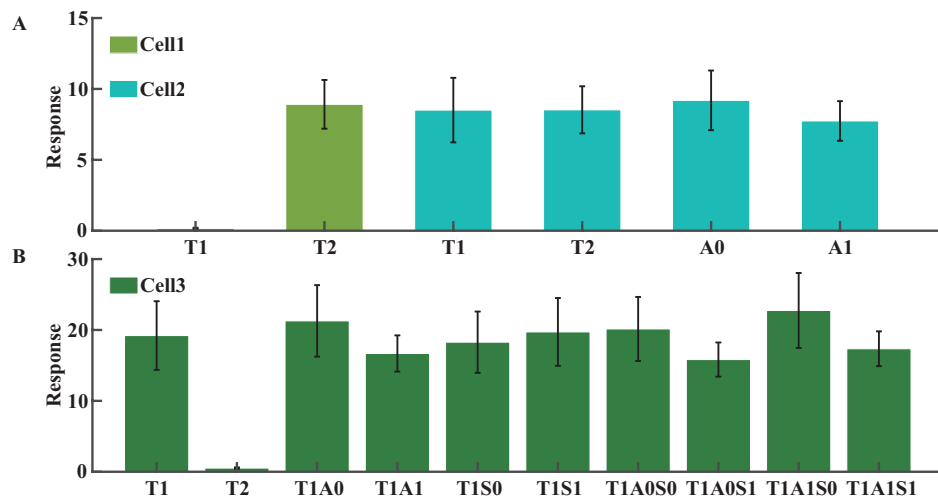

**Figure S2. Mixed selectivity of neurons in the PFC-analogous layer in context-dependent processing.** Before the analysis, the network was sequentially trained to perform two tasks depending on the contextual information. Task 1 (T1): to classify if a face is attractive (A1) or not (A0). Task 2 (T2): to classify if a face is smiling (S1) or not (S0). The data are presented as mean  $\pm$  s.d across all correctly classified images.

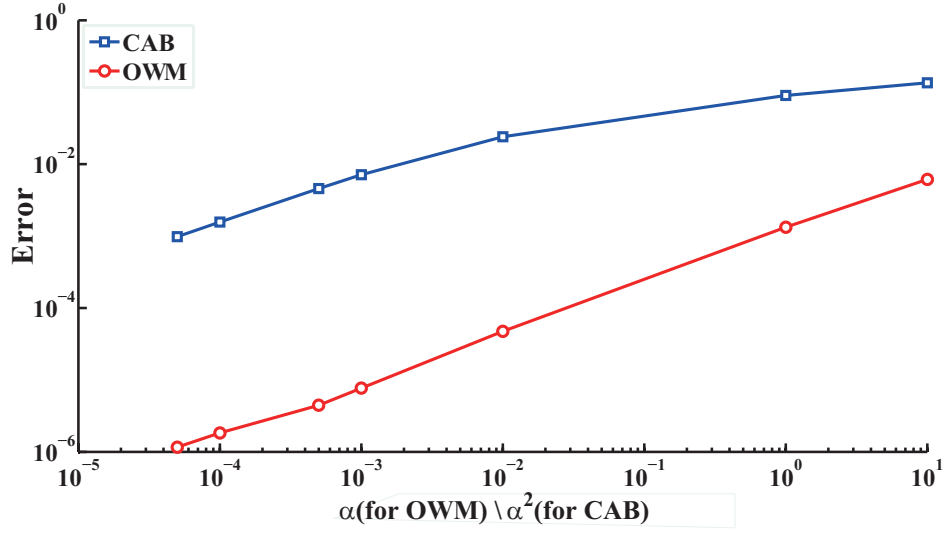

**Figure S3.** The error between the original inputs and projected inputs by CAB and OWM with respect to different parameters. Note that the parameter  $\alpha^2$  (for CAB) and  $\alpha$  (for OWM) is not related, so one is not the square (or square root) of the other.

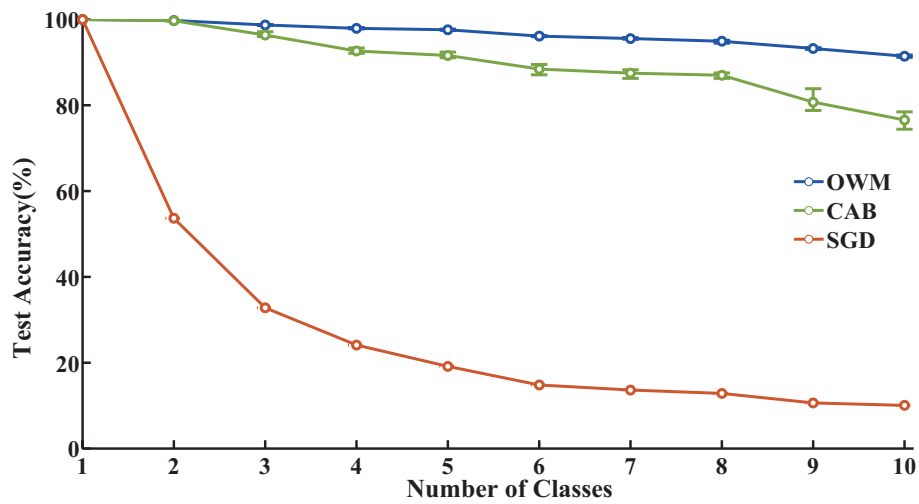

**Figure S4.** The performance of the OWM, CAB, and a fine-tuned baseline (SGD) in the 10-disjoint MNIST task, in which 10 digits, from 0 to 9, were learned sequentially. The test accuracy was plotted as a function of number of classes learned. The results were presented as mean  $\pm$  s.d. across ten experiments.

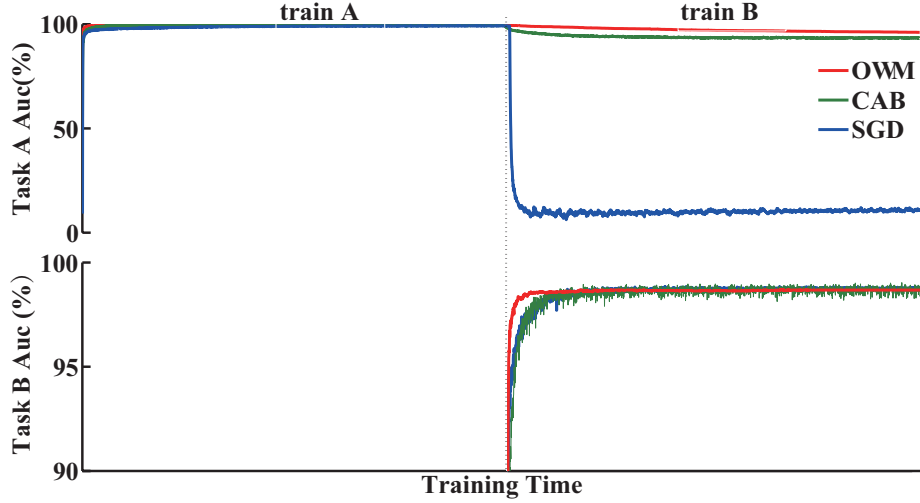

**Figure S5.** The learning curves in the 2-disjoint MNIST task for the methods of OWM, CAB and SGD. The Task A was to recognize the digits from 0 to 4, while the Task B was to recognize the digits form 5 to 9.

| Shuffled MNIST Experiment |                                  |                                         |                  |
|---------------------------|----------------------------------|-----------------------------------------|------------------|
| 3 tasks                   | Accuracy (%)                     | 10 tasks                                | Accuracy (%)     |
| SGD <sup>#</sup> [7]      | 71.32 $\pm$ 1.54*                | EWC <sup>#</sup> [8]                    | $\sim$ 97.0      |
| IMM <sup>#</sup> [9]      | 98.30 $\pm$ 0.08 <sup>n.s.</sup> | <b>OWM</b> <sup>#</sup>                 | 97.52 $\pm$ 0.03 |
| EWC <sup>#</sup> [8]      | $\sim$ 98.2                      | EWC <sup>†</sup> [5]                    | $\sim$ 89.0      |
| <b>OWM</b> <sup>#</sup>   | 98.34 $\pm$ 0.02                 | CAB <sup>†</sup> [5]                    | $\sim$ 95.2      |
|                           |                                  | OWM <sup>†</sup>                        | 95.15 $\pm$ 0.08 |
|                           |                                  | Synaptic Intelligence <sup>‡</sup> [10] | $\sim$ 97.2      |
|                           |                                  | <b>OWM</b> <sup>‡</sup>                 | 97.64 $\pm$ 0.03 |

**Table S1. Comparison of the performance of different methods in the Shuffled MNIST task.** Network size: <sup>†</sup>, 3-layer networks with [784-800-10] neurons; <sup>#</sup>, 4-layer networks with [784-800-800-10] neurons; <sup>‡</sup>, 4-layer networks with [784-2000-2000-10] neurons. The results for others methods were adopted from corresponding publications. The results for OWM are represented as mean  $\pm$  s.d. across 10 experiments. The L2 regularization coefficient was 0.001. Dropout was applied for all methods tested above, with the drop rate of 0.2. \*,  $p < 0.01$ , two-sides t test, compared to the results of OWM achieved with the same network size. n.s, not significant.

| Disjoint MNIST Experiment |                   |
|---------------------------|-------------------|
| Methods                   | Accuracy (%)      |
| EWC <sup>#</sup> [9]      | 52.72 $\pm$ 1.36* |
| IMM <sup>#</sup> [9]      | 94.12 $\pm$ 0.27* |
| <b>OWM</b> <sup>#</sup>   | 96.71 $\pm$ 0.11  |
| SGD <sup>†</sup>          | 53.85 $\pm$ 0.14* |
| CAB <sup>†</sup> [5]      | 94.91 $\pm$ 0.30* |
| <b>OWM</b> <sup>†</sup>   | 96.51 $\pm$ 0.10  |

**Table S2. Comparison of the performance of different methods in the Disjoint MNIST task.** Network size: <sup>†</sup>, 3-layer networks with [784-800-10] neurons; <sup>#</sup>, 4-layer networks with [784-800-800-10] neurons. The performance of approaches other than OWM was adopted from previously published results 12. The results for OWM are represented as mean  $\pm$  s.d. across 10 experiments. The L2 regularization coefficient was 0.0001. In the second task, the learning rates for all but the output layer were reduced to 0.01. \*,  $p < 0.01$ , two-sides t test, compared to the results of OWM achieved with the same network size.

| Attributes | 5 Shadow       | Arched E.Brows | Attractive | Bags Un.Eyes | Bald          | Bangs        | Big Lips      | Big Nose         | Black Hair    | Blond Hair    | Blurry       | Brown Hair | Bush E.Brows | Chubby      |
|------------|----------------|----------------|------------|--------------|---------------|--------------|---------------|------------------|---------------|---------------|--------------|------------|--------------|-------------|
| ST         | 94.66          | 83.80          | 82.77      | 85.29        | 98.96         | 96.16        | 71.37         | 84.37            | 90.32         | 96.13         | 96.12        | 89.85      | 92.81        | 95.71       |
| MT         | 94.82          | 83.83          | 83.01      | 85.28        | 90.00         | 96.27        | 71.66         | 84.89            | 90.55         | 96.10         | 96.28        | 89.56      | 92.95        | 95.83       |
| Attributes | Double Chin    | Eyeglasses     | Goatee     | Gray Hair    | Heavy Makeup  | H.Cheekbones | Male          | Mouth Small Open | Mustache      | Narrow Eyes   | No Beard     | Oval Face  | Pale Skin    | Pointy Nose |
| ST         | 96.36          | 99.67          | 97.56      | 98.37        | 91.87         | 87.94        | 98.56         | 94.05            | 97.01         | 87.29         | 96.27        | 75.62      | 97.04        | 77.18       |
| MT         | 96.41          | 99.67          | 97.67      | 98.36        | 91.98         | 87.96        | 98.56         | 93.99            | 97.08         | 87.35         | 96.28        | 75.91      | 97.25        | 77.44       |
| Attributes | Reced.Hairline | Rosy Cheeks    | Sideburns  | Smiling      | Straight Hair | Wavy Hair    | Wear Earrings | Wear Hat         | Wear Lipstick | Wear Necklace | Wear Necktie | Young      | Average      |             |
| ST         | 93.79          | 95.13          | 97.90      | 93.22        | 84.59         | 84.99        | 90.58         | 99.10            | 94.28         | 87.08         | 96.50        | 88.61      | <b>91.47</b> |             |
| MT         | 93.97          | 95.12          | 97.88      | 93.13        | 84.60         | 85.05        | 90.70         | 99.15            | 94.32         | 87.11         | 96.61        | 88.69      | <b>91.56</b> |             |

**Table S3. Performance of OWM in context-dependent, sequentially learning, compared with the results obtained by multi-task training, in detecting 40 different facial attributes in CelebA. MT, multi-task training; ST, sequential training with OWM.**

| Hyperparameters of different Feature Extractor |                               |               |              |            |
|------------------------------------------------|-------------------------------|---------------|--------------|------------|
| Experiment                                     | Feature Extractor/Output Size | Learning Rate | Weight Decay | Batch Size |
| ImageNet ILSVR2012                             | ResNet152 / 2048              | 0.1           | 0.0001       | 512        |
| CASIA-HWDB1.1                                  | ResNet18 / 1024               | 0.1           | 0.0001       | 512        |
| CelebA                                         | ResNet50 / 2048               | 0.1           | 0.0001       | 256        |

**Table S4. Hyperparameters of the feature extractors used in different tasks.** ResNet was adopted from [11]. The optimization method of all feature extractor were RMSprop [12].

| Hyperparameters of different method |          |          |               |            |
|-------------------------------------|----------|----------|---------------|------------|
| Experiment                          | $\alpha$ | $\kappa$ | Learning Rate | Batch Size |
| Shuffled MNIST                      | 1        | 1.8      | NA            | 100        |
| Disjoint MNIST                      | 0.1      | 1        | NA            | 30         |
| Disjoint MNIST(SGD)                 | NA       | NA       | 0.01          | 50         |
| ImageNet ILSVR2012                  | 0.2      | $c$      | NA            | 50         |
| ImageNet ILSVR2012(SGD)             | NA       | NA       | 0.01          | 1000       |
| CASIA-HWDB1.1                       | 0.2      | $c$      | NA            | 10         |
| CASIA-HWDB1.1(SGD)                  | NA       | NA       | 0.01          | 100        |
| CelebA                              | 0.2      | $c$      | NA            | 10         |

**Table S5. Hyperparameters for OWM/SGD method used in different experiments.**  $c = \frac{1}{1+\mathbf{x}^T\mathbf{P}\mathbf{x}}$ .
